# Supplementary material for: Learner-aware Teaching: Inverse Reinforcement Learning with Preferences and Constraints
Source: arXiv:1906.00429 source file (2019-10-29)
Supplement: Supplementary file 1 [file 9.6_appendix_limit_learner.tex]

\section{Limit Learner \todo{title}}
\label{appendix:limit-learner}

To understand the relationship between the teacher's provided demonstrations and learner's identified policy (and induced feature expectations), as well as the resulting sub-optimality, we study a learner parameterized by $C_r$ of the form:
\begin{align}
\max_{\pi, \delta^{\textnormal{soft}}_r} \qquad &H(A_{0:\infty} \Vert S_{0:\infty}) - C_r \cdot \| \delta^{\textnormal{soft}}_r \|_2 \\
\textnormal{subject to}\nonumber\\
&\lvert \mu_{r,i}(\pi) - \hat{\mu}_{r,i}(\Xi^{\mathscr{T}}) \rvert \leq \delta^{\textnormal{soft}}_{r,i} \ \forall i \in \{1, 2, \ldots, d_r\} \\
&g_j(\mu_{c}(\pi)) \leq \delta^{\textnormal{hard}}_{c,j} \ \forall j \in \{1, 2, \ldots, m\}
\end{align}
We are particularly interested in studying the case $C_r \rightarrow \infty$, intuitively corresponding to a case in which the learner puts his main emphasis on matching the teacher's demonstrations as closely as possible while satisfying the preference constraints.
For an optimal solution of the above problem, $\lvert \mu_{r,i}(\pi) - \hat{\mu}_{r,i}(\Xi^{\mathscr{T}}) \rvert = \delta^{\textnormal{soft}}_{r,i}$ and the objective becomes
$\max_{\pi} \; H(A_{0:\infty} \Vert S_{0:\infty}) - C_r \cdot \| \mu_{r,i}(\pi) - \hat{\mu}_{r,i}(\Xi^{\mathscr{T}}) \|_2$.
We distinguish the following two relevant cases:
\begin{itemize}
  \item \textbf{Learner can't match the teacher's feature expectation} ($\hat{\mu}_{r,i}(\Xi^{\mathscr{T}}) \not\in \Omega_c$). Note that since the optimal solution of an optimization problem is unchanged under scaling of the objective by a scalar, we can rewrite the objective as $\max_{\pi} \; \tfrac{1}{C_r} H(A_{0:\infty} \Vert S_{0:\infty}) - \| \mu_{r,i}(\pi) - \hat{\mu}_{r,i}(\Xi^{\mathscr{T}}) \|_2$.
  Since the entropy in the objective is bounded, in the limit $C_r \rightarrow \infty$, the problem will converge to the  projection of $\hat{\mu}_{r,i}(\Xi^{\mathscr{T}})$ onto $\Omega_c$.
  
  \item \textbf{Learner can match the teacher's feature expectation} ($\hat{\mu}_{r,i}(\Xi^{\mathscr{T}}) \in \Omega_c$). In this case, in the limit $C_r \rightarrow \infty$, the learner outputs a policy which maximizes causal entropy, exactly matches the teacher's feature expectation and satisfies the preference constraints.
\end{itemize}
Hence, in the limit, the learner solves the problem
\begin{align}
\max_{\pi} \qquad &H(A_{0:\infty} \Vert S_{0:\infty}) \\
\textnormal{subject to}\nonumber\\
&  \mu_{r}(\pi) = \textnormal{Proj}_{\Omega_c}(\hat{\mu}_{r}(\Xi^{\mathscr{T}})) \\
&g_j(\mu_{c}(\pi)) \leq \delta^{\textnormal{hard}}_{c,j} \ \forall j \in \{1, 2, \ldots, m\},
\end{align}
where $\textnormal{Proj}_{\Omega_c}(\mu)$ denotes the Euclidean projection of $\mu$ onto $\Omega_c$.
