# Supplementary material for: Learner-aware Teaching: Inverse Reinforcement Learning with Preferences and Constraints
Source: arXiv:1906.00429 source file (2019-10-29)
Supplement: Supplementary file 2 [file 9.7_appendix_known.tex]

%!TEX root = main.tex

\section{Further Experimental Results: Known Learner Preferences}
\label{appendix:experiments-known-learner}
